# Supplementary material for: A Quantum Approximate Optimization Method For Finding Hadamard Matrices
Source: arXiv:2408.07964 source file (2024-10-13)
Supplement: Supplementary file 1 [file Appendix.tex]

\appendix
%Supplementary Information
%\appendix
%\newpage
\section{Representative problems for each $k$-body cases}
In this section, we will evaluate and validate each of the k-body circuits with a simple problem of finding low order H-matrix before employing them into the full problem. The prototypical problem is finding a 2-order H-matrix, where the unknown entries will subsequently be increased to represent the increasing number of interaction $k$ for the $k$-body terms.

%\subsubsection{Elementary cases}
\subsection{1-body}
% -- 1-Body, QAOA ------
\begin{figure*}[h!]
    \centering
    \subfloat[\centering A quantum circuit for 2-qubits QAOA problem]
    {{\includegraphics[width=0.6\columnwidth]{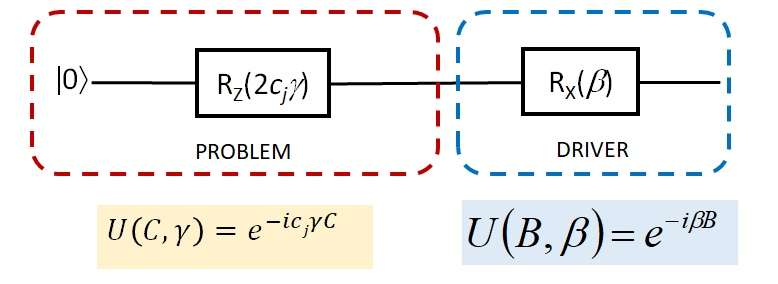} }}%
    %\qquad
    \\
    \subfloat[\centering Realized Quantum Circuit in Qiskit]
    {{\includegraphics[width=0.45\columnwidth]{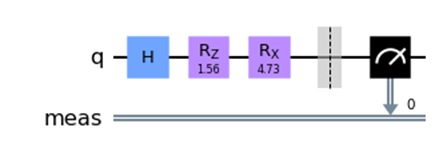} }} %
    \subfloat[\centering Distribution of solution]
    {{\includegraphics[width=0.45\columnwidth]{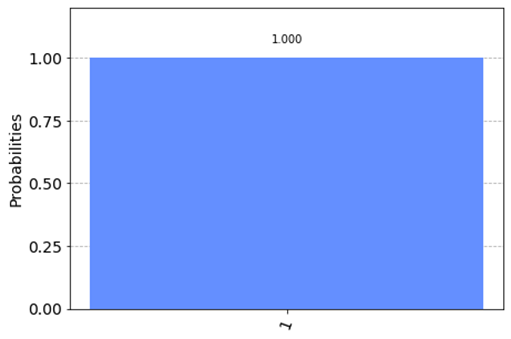} }} %
    %%--
    \caption{ Quantum Circuit for 1-body Interaction}%
    \label{FIG_1BODYX}%
\end{figure*}
The first case to consider is the problem involving only 1-body terms. A representative problem of finding 2-order H-matrix with 1 unknown can be formulated as follows
\begin{equation}
    \nonumber
    \begin{pmatrix}
        1 & 1  \\
        1 & s_1
    \end{pmatrix}
\end{equation}

The related energy function as formulated in Eq.(\ref{EQ_QAOA_problem}) is then given by

\begin{equation}
    E=2(1+s_1)
    \label{EQ_1body_hsearch}
\end{equation}
whose corresponding Hamiltonian is 
\begin{equation}
    \hat{H}\left( \hat{\sigma}\right)=2\left(1+\hat{\sigma}^z_{1}\right) 
    \label{EQ_1body_hsearch_hamiltonian}
\end{equation}
It is obvious that the solution will be $s_1 = -1$, which in the binary variable domain is equal to "1" (remind that the spin-to-binary variable transform is: $"0" \leftrightarrow  1, "1" \leftrightarrow -1$). The corresponding QAOA circuit can be constructed after insertion of driver Hamiltonian represented as an X-rotation of angle $\beta$, which is shown in Fig.\ref{FIG_1BODYX}(a). After constructing the circuit and running the program, we obtain the results shown in Fig. \ref{FIG_1BODYX} (b) and (c).

We can calculate the performance of this algorithm as follows. Since there is only one variable, a random algorithm will output a single bit string, therefore are two possibilities of the output, which are "0" and "1". The probability of the solution in the random algorithm is $P_R=\frac{1}{2}=0.5$. On the other hand, the quantum algorithm gives one correct answer so that $P_A=1.0$ as shown in the histogram. Accordingly, we have $xRR=\frac{P_A}{P_R} = 2$.

\subsection{2-body}
% -- 2-Body, QAOA ------
\begin{figure*}[h!]
    \centering
    \subfloat[\centering A quantum circuit for 2-qubits QAOA problem]
    {{\includegraphics[width=0.6\columnwidth]{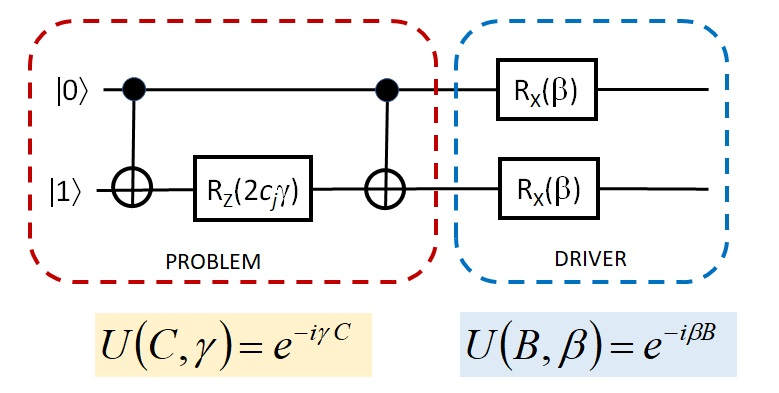} }}%
    %\qquad
    \\
    \subfloat[\centering Realized Quantum Circuit in Qiskit]
    {{\includegraphics[width=0.45\columnwidth]{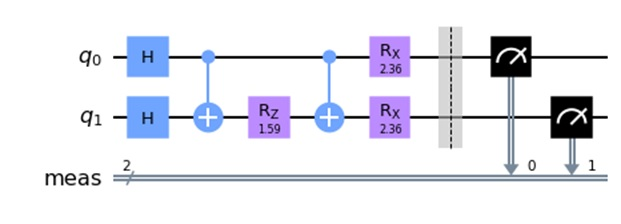} }} %
    \subfloat[\centering Distribution of solution]
    {{\includegraphics[width=0.45\columnwidth]{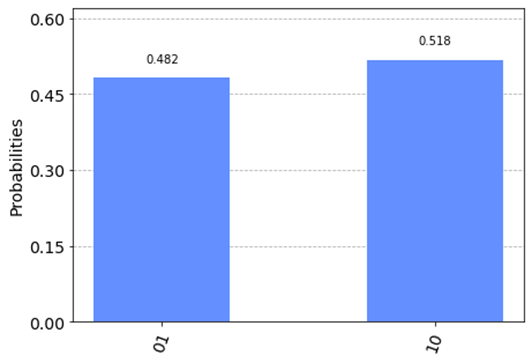} }} %
    \caption{QAOA circuits and simulation results of 2-qubits problem}%
    \label{FIG_2BODYX}%
\end{figure*}
%
% --- need related simulations on quantum simulator ---
The prototypical problem for a 2-body case can be formulated similarly, but now we have two variables $s_1, s_2$. We can formulate the searched matrix as follows
\begin{equation}
    \nonumber
    \begin{pmatrix}
        1 & s_1  \\
        1 & s_2
    \end{pmatrix}
\end{equation}

The energy function related to this problem is therefore
\begin{equation}
    E=(s_1+s_2)^2 = 2(1+s_1s_2)
    \label{EQ_2body_hsearch}
\end{equation}
whose corresponding Hamiltonian is 
\begin{equation}
    \hat{H}\left( \hat{\sigma}\right)=2\left(1+\hat{\sigma}^z_{1}\hat{\sigma}^z_{2} \right) 
    \label{EQ_2body_hsearch_hamiltonian}
\end{equation}
the simplification is obtained since we know that $s_i \in {-1,1}$ implying $s_i^2=1$. Obviously, the solution in the binary form will be either "01" or "10". The quantum circuit for this problem is given by Fig. \ref{FIG_2BODYX} (a). 

Running the circuit into a simulator of quantum processor gives the following result displayed in Fig.\ref{FIG_2BODYX} (b) and its histogram in (c). The histogram of the simulation results shows that the solution is distributed almost equally into "01" and "10", as expected. Since the output is a 2-bit strings and there are 2 valid solutions, the probability of the solution by the random algorithm is $P_R=\frac{2}{4}=\frac{1}{2}=0.5$. From Fig. Fig.\ref{FIG_2BODYX} (c) we have $P_A=0.482+0.518 = 1.0$; therefore $xRR=\frac{1}{0.5}=2$.

\subsection{3-body}
% -- 3-Body, QAOA ------
\begin{figure*}[h!]
    \centering
    \subfloat[\centering A quantum circuit for 3-qubits QAOA problem]
    {{\includegraphics[width=0.6\columnwidth]{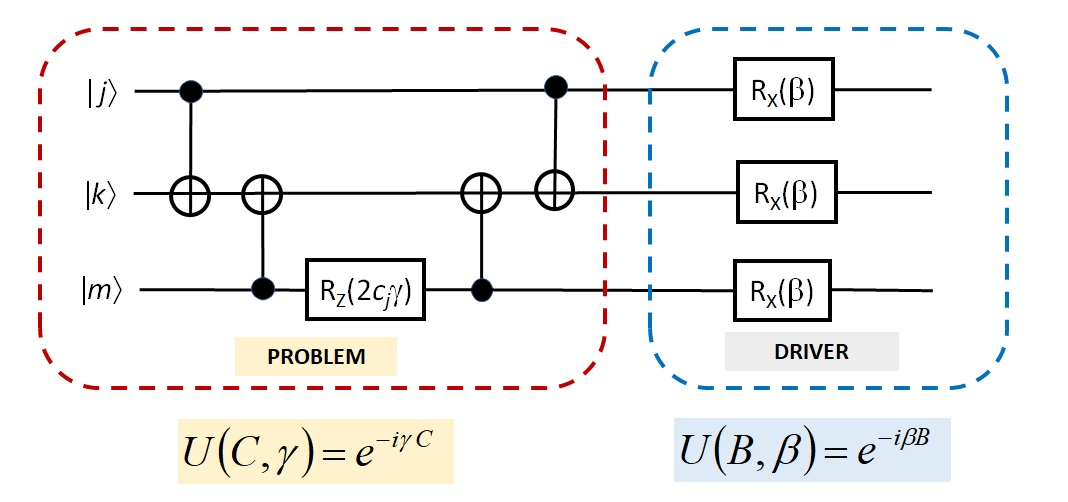} }}%
    %\qquad
    \\
    \subfloat[\centering Realized Quantum Circuit in Qiskit]
    {{\includegraphics[width=0.45\columnwidth]{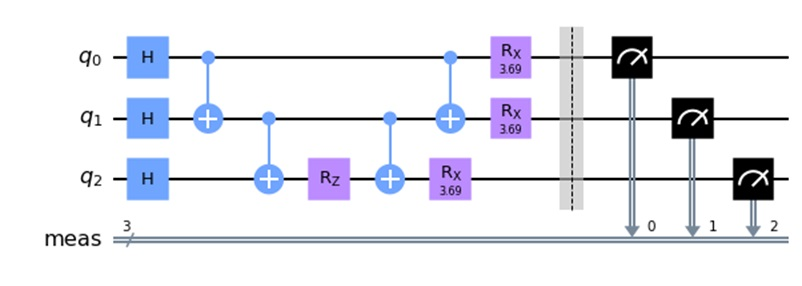} }} 
    \subfloat[\centering Distribution of solution]
    {{\includegraphics[width=0.45\columnwidth]{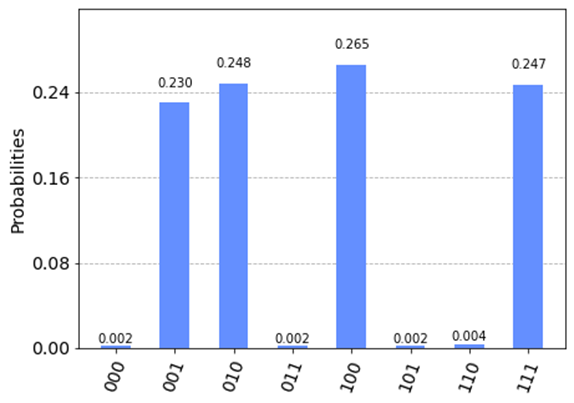} }} %
    %% -- 
    \caption{QAOA circuits and simulation results of 3-qubits problem}%
    \label{FIG_3BODYX}%
\end{figure*}
The 3-body prototypical problem can be represented by 3-unknown entries with corresponding variables $s_1, s_2, s_3$ in the 2-order H-matrix as follows

\begin{equation}
    \nonumber
    \begin{pmatrix}
        1 & s_1  \\
        s_2 & s_3
    \end{pmatrix}
\end{equation}

The related energy function can be computed similarly, which gives the following expression 
\begin{equation}
    E=(s_1+s_2s_3)^2 = 2(1+s_1s_2s_3)
    \label{EQ_3body_hsearch}
\end{equation}
whose corresponding Hamiltonian is 
\begin{equation}
    \hat{H}\left( \hat{\sigma}\right)=2\left(1+\hat{\sigma}^z_{1}\hat{\sigma}^z_{2} \hat{\sigma}^z_{3} \right) 
    \label{EQ_3body_hsearch_hamiltonian}
\end{equation}
The quantum circuit for this problem is displayed in Fig. \ref{FIG_3BODYX} (a). Then, we run the circuit in quantum simulator and get the following results shown in Fig.\ref{FIG_3BODYX} (b) and  (c). The histogram in (c) shows the peak distributions into 4 cases corresponding with solution of "001", "010", "100", and "111". Considering bit "1" represents "-1" spin-value, all of the peaks are correct solutions. Since the output is a 3-length bitstrings, the probability of the solution in a random algorithm is $P_R=4\frac{1}{8}=\frac{1}{2}=0.5$, whereas the probability of the solution by the quantum algorithm as shown in the histogram is $P_A=0.230+0.248+0.265+0.247=0.99$. Therefore, the performance metric is $xRR=\frac{0.99}{0.5}= 1.98$.

% -- 4-Body, QAOA ------
\begin{figure*}[h!]
    \centering
    \subfloat[\centering A quantum circuit for 4-qubits QAOA problem]
    {{\includegraphics[width=0.6\columnwidth]{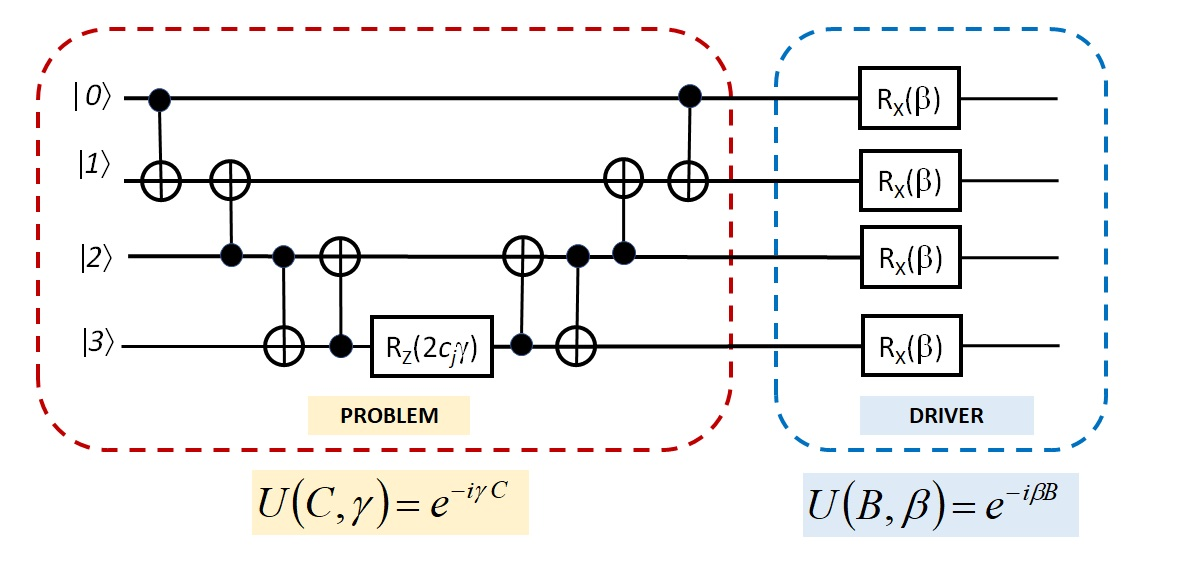} }}%
    %\qquad
    \\    
    \subfloat[\centering Realized Quantum Circuit in Qiskit]
    {{\includegraphics[width=0.45\columnwidth]{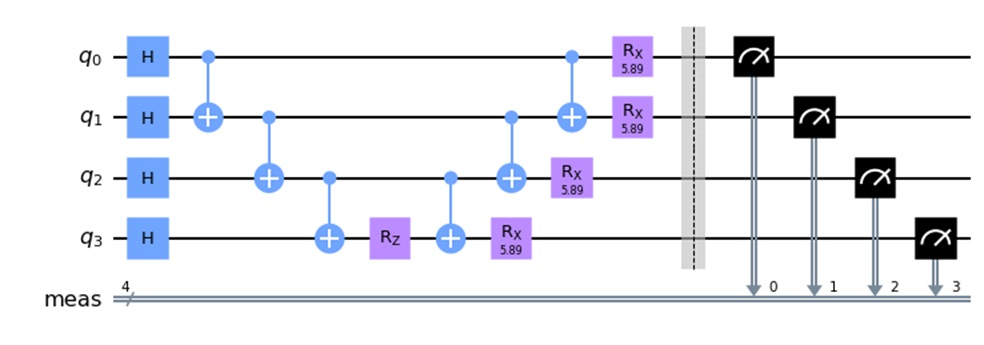} }} 
    \subfloat[\centering Distribution of solution]
    {{\includegraphics[width=0.45\columnwidth]{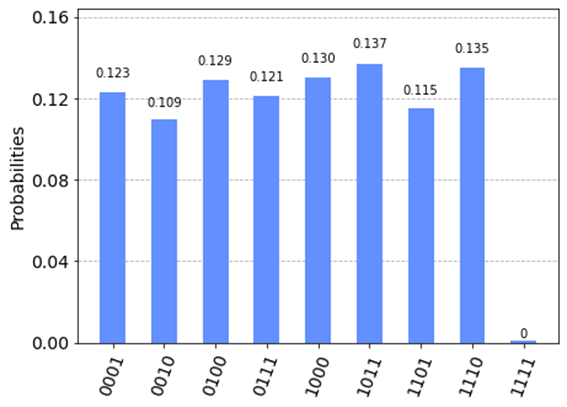} }} %
    \caption{QAOA circuits and simulation results of 4-qubits problem}%
    \label{FIG_4BODYX}%
\end{figure*}

\subsection{4-body}
%The last case is 4-body interactions. 
The matrix related to 4-body interaction is given as follows,
%We did the experiment with two cases, i.e., 4-body embedded in a 2-order H-matrix and in a 4-order H-matrix. 
%For the first case, the 2-order H-matrix is given as follows
\begin{equation}
    \nonumber
    \begin{pmatrix}
        s_1 & s_3  \\
        s_2 & s_4
    \end{pmatrix}
\end{equation}
with energy related function is given by
\begin{equation}
    E=(s_1s_3+s_2s_4)^2 = 2(1+s_1s_2s_3s_4)
    \label{EQ_4body_hsearch}
\end{equation}
whose corresponding Hamiltonian is given by
\begin{equation}
    \hat{H}\left( \hat{\sigma}\right)=2\left(1+\hat{\sigma}^z_{1}\hat{\sigma}^z_{2} \hat{\sigma}^z_{3}\hat{\sigma}^z_{4} \right) 
    \label{EQ_4body_hsearch_hamiltonian}
\end{equation}
The quantum circuit for this problem is given by Fig. \ref{FIG_4BODYX} (a).

We run the circuit in quantum simulator and get the following results shown in Fig.\ref{FIG_4BODYX}(b) and (c). The histogram in (c) shows the peak distributions into 4 cases corresponding with solution of "0001", "0010", "0100", "0111", "1000", "1011", "1101", and "1110", all of them are correct solutions. The probability of correct solution in a random algorithm will be $P_R=8\frac{1}{2^4}=0.5$, whereas the probability of the quantum algorithm is $P_A=0.123+0.109+0.129+0.121+0.130+0.137+0.115+0.135=0.999$. Therefore, the performance metric is $xRR=\frac{P_A}{P_R} = \frac{0.999}{0.5}=1.998$.

\section{Cascaded $k$-body cases}
The previous subsection presents experiments of individual $k$-body cases, which are the simplest case involving Problem Hamiltonian with only one term. In this subsection, we present the experiments results when the terms are unified. Some sub cases will be considered, which are: (a) uniform $k$-body and with uniform coefficients, (b) uniform $k$-body with non-uniform coefficients, and (c) mixed $k$-body. We minimize the mean error of the objective function by using the COBYLA (Constrained Optimization BY Linear Approximatio) method provided in Pyhton package. The initial values of the parameters $\{\gamma, \beta \}$ are set at random.

% -- uniform 2-body, uniform coeffs------
\begin{figure*}[h!]
    \centering
    \subfloat[\centering Iteration curve for $p=1$]
    {{\includegraphics[width=0.45\columnwidth]{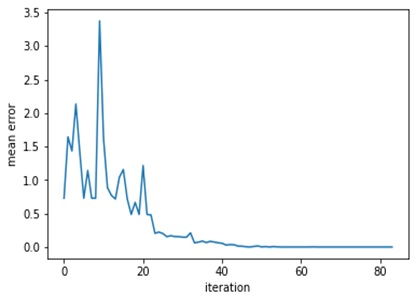} }}%
    %\qquad    
    \subfloat[\centering Distribution of solution for $p=4$]
    {{\includegraphics[width=0.45\columnwidth]{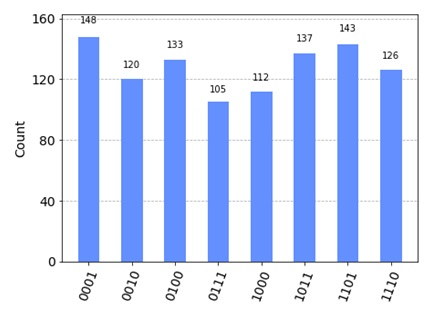} }} 
    \\
    \subfloat[\centering Quantum Circuit $p=1$]
    {{\includegraphics[width= 1.0\columnwidth]{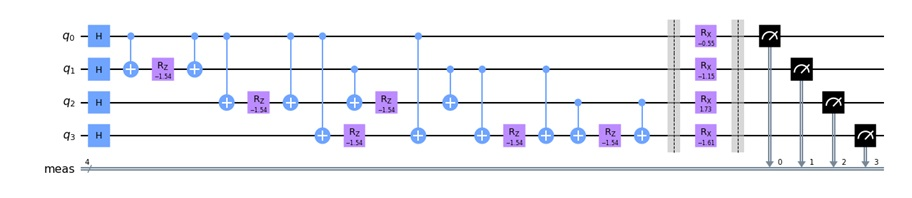} }}%
    
    \caption{Uniform 2-Body with Uniform Coefficients}%
    \label{FIG_2body_uniform_coeffs}%
\end{figure*}
%

%/////////////////////////////////////////////////////////////
\subsection{Case-1: 2-body terms with uniform coefficients}
%/////////////////////////////////////////////////////////////
The Hamiltonian terms in this case are similar to the max-cut problem. Here, we define a Hamiltonian that is not related particularly to the Hadamard matrix problem. All of the terms are 2-body interactions, which is given by

\begin{equation}
    H_P= s_0s_1 + s_0s_2 + s_0s_3 + s_1s_2 + s_1s_3 + s_2s_3
    \label{EQ_2body_uniform_coeffs}
\end{equation}

Since there ae 4 binary variables, the number of total possible output is 16. An exhaustive check shows that there are 8 bit strings of correct solutions, which are $\{0001, 0010, 0100, 0111, 1000, 1011, 1101, 1110\}$. This give the probability of random algorithm $P_R=\frac{8}{16}=\frac{1}{2}$. 

We found that running QAOA on a simulator with $p=1$ is sufficient to find all solutions. The simulation results are displayed in Fig.\ref{FIG_2body_uniform_coeffs}, with (a) the iteration curve, (b) distribution of solution, and (c) quantum circuit of the problem. The quantum circuit shown in (c) is similar to the QAOA of maxcut problems [REF-IBM-qiskit-book]. The final objective functions reach the absolute minimum of $0.000$ and all of $1024$ shots gives a correct solutions which corresponds to $P_A=1.000$. Accordingly, the performance is $xRAR=\frac{P_A}{P_R}=2.000$.

% -- uniform 2-body, non-uniform coeffs------
\begin{figure*}[h!]
    \centering
    \subfloat[\centering Iteration curve for $p=1$]
    {{\includegraphics[width=0.45\columnwidth]{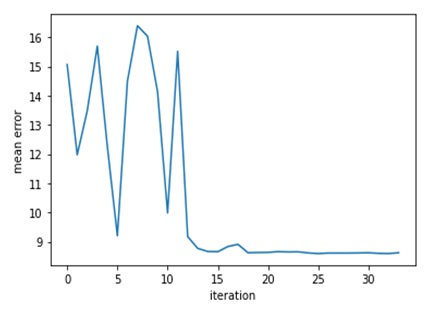} }}%
    %\qquad    
    \subfloat[\centering Distribution of solution for $p=1$]
    {{\includegraphics[width=0.45\columnwidth]{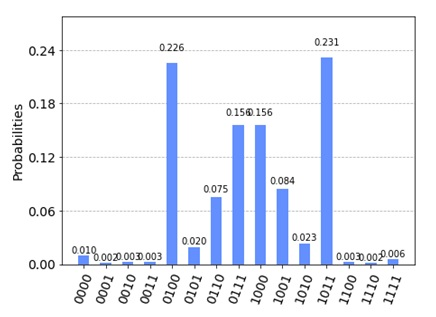} }} 
    \\
    \subfloat[\centering Quantum Circuit $p=1$]
    {{\includegraphics[width= 1.0\columnwidth]{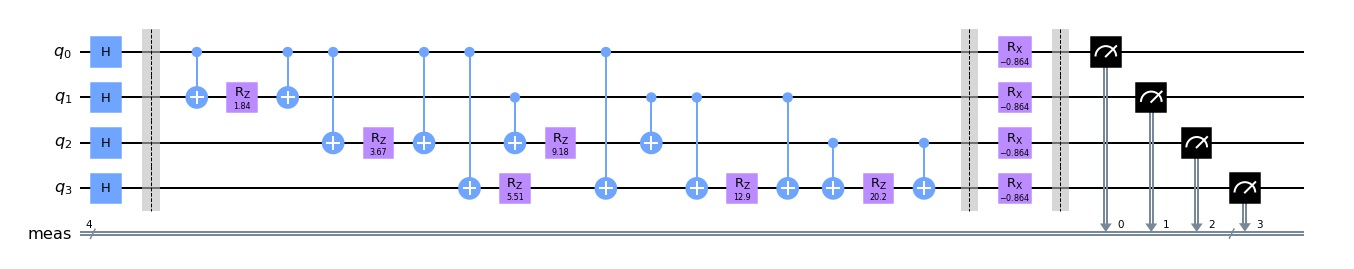} }}%
    
    \caption{Uniform 2-Body with Non-Uniform Coefficients}%
    \label{FIG_2body_non_uniform_coeffs_01}%
\end{figure*}
%
%/////////////////////////////////////////////////////////////
\subsection{Case-2: 2-body with non-uniform coefficients}
%/////////////////////////////////////////////////////////////
In this experiment, the Hamiltonian of the problem is given by the following 
\begin{equation}
    H_P= s_0s_1 + 2s_0s_2 + 3s_0s_3 + 5s_1s_2 + 7s_1s_3 + 11s_2s_3 -3
    \label{EQ_2body_non_uniform_coeffs}
\end{equation}
The constant $3$ in this equation is an offset that makes the absolute minimum value of $H_P$ equal to zero. This equation Eq.(\ref{EQ_2body_uniform_coeffs}) is slightly different from Eq.(\ref{EQ_2body_non_uniform_coeffs}), all terms are two-bodies but with several different  coefficients in the later. The total number of possible output is also 16, but the correct solutions is 2; which are $\{0100, 1011\}$ this gives $P_R=\frac{1}{8}$. 

We do the experiment by increasing the number of layers $p$. The results are displayed in Fig. \ref{FIG_2body_non_uniform_coeffs_01} and Fig. \ref{FIG_2body_non_uniform_coeffs_02}, which shows increasing performance in terms of increasing xRAR and decreasing objective error. The table in Fig. \ref{FIG_2body_non_uniform_coeffs_02} (c) clearly shows increasing performance with increasing number of layers.

% -- uniform 2-body, non-uniform coeffs:: FIG-2------
\begin{figure*}[h!]
    \centering
    \subfloat[\centering Iteration curve for $p=2NQ^2$]
    {{\includegraphics[width=0.45\columnwidth]{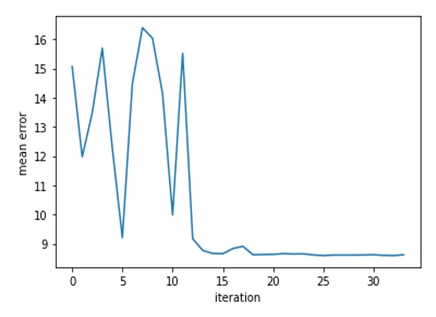} }}%
    %\qquad    
    \subfloat[\centering Distribution of solution for $p=1$]
    {{\includegraphics[width=0.45\columnwidth]{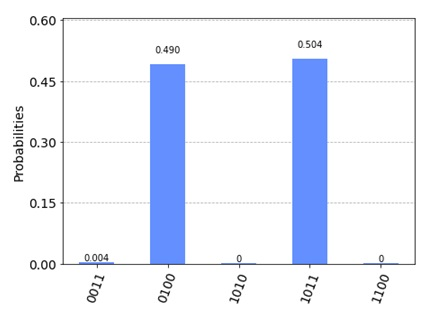} }} 
    \\
    \subfloat[\centering Performance Table]
    {{\includegraphics[width= 0.5\columnwidth]{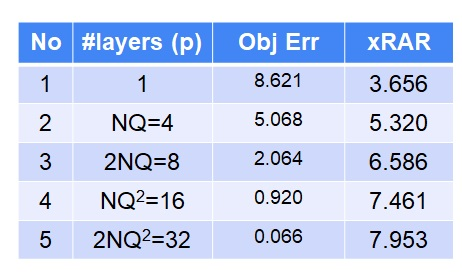} }}%
    
    \caption{Uniform 2-Body with Non-Uniform Coefficients: high layer number and table of performance}%
    \label{FIG_2body_non_uniform_coeffs_02}%
\end{figure*}

\subsection{Case-3: mixed $k$-body, uniform coefficients}
In this case, we have the following problem Hamiltonian
\begin{equation}
    \label{EQ_mixed_k_body_uniform_coeffs_hamiltonian}
    H_P= s_0 + s_1 + s_2 + s_0s_1 + s_1s_2 + s_1s_2s_3 + s_0s_1s_2s_3-1
\end{equation}

There are 4 valid bit string solutions, which are $\{0101, 0110, 1000, 1001\}$, so that $P_R=\frac{1}{4}$. Simulation results are shown in Fig.\ref{FIG_kbody_uniform_coeffs}. The distribution in (b) shows dominant probability on the solutions, while the table in (c) shows increasing performance with increasing $p$.

% -- mixed k-body, uniform coeffs
\begin{figure*}[h!]
    \centering
    \subfloat[\centering Distribution of solution for $p=1$]
    {{\includegraphics[width=0.45\columnwidth]{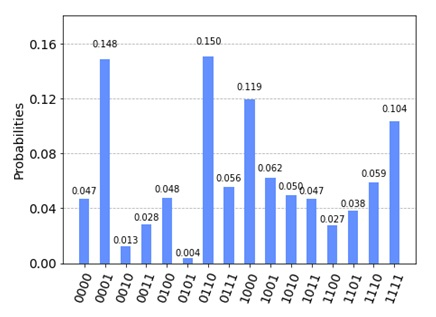} }} 
    \subfloat[\centering Distribution of solution for $p=2(NQ)^2$]
    {{\includegraphics[width=0.45\columnwidth]{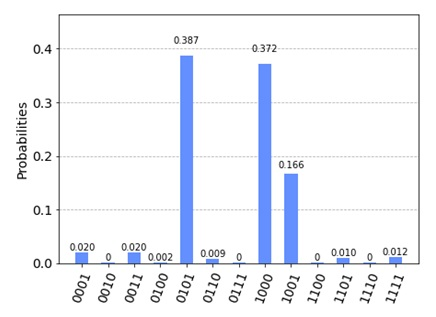} }} 
    \\
    \subfloat[\centering Iteration curve for $p=2(NQ)^2$]
    {{\includegraphics[width=0.48\columnwidth]{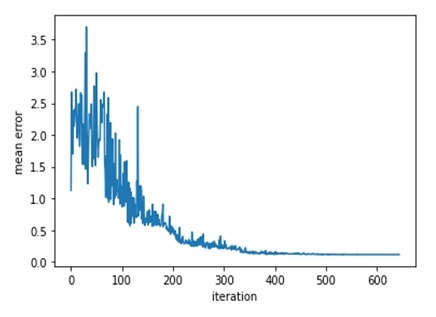} }}%
    %\qquad    
    \subfloat[\centering Performance Table]
    {{\includegraphics[width= 0.48\columnwidth]{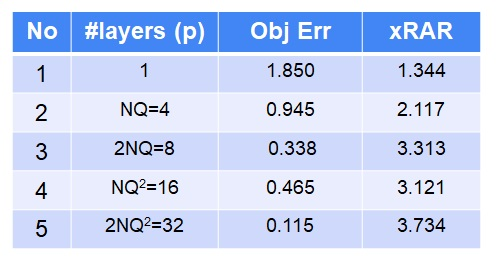} }}%
    \caption{Mixed k-Body with Uniform Coefficients}%
    \label{FIG_kbody_uniform_coeffs}%
\end{figure*}

\subsection{Case-4: mixed $k$-body, non-uniform coefficients}
The problem Hamiltonian for mixed $k$-body with non uniform coefficients is as follows,
\begin{equation}
    \label{EQ_mixed_k_body_uniform_coeffs_hamiltonian}
    H_P= s_0 + 2s_1 + 3s_2 + 5s_0s_1 + 7s_1s_2 + 11s_1s_2s_3 + 13s_0s_1s_2s_3
\end{equation}

There is only one valid bit string for this problem, which is $1100$, so that the probability of random algorithm is $P_R=16$. Some of the simulation results are displayed in Fig.\ref{FIG_kbody_non_uniform_coeffs}. In part (b) and (c), we observe re-concentration of distribution toward the solution at higher value of $p$. The performance table in (d) shows that increasing $p$ tends to iprove the performance, although at some value of $p$ it can reduced.

% -- mixed k-body, non-uniform coeffs
\begin{figure*}[h!]
    \centering
    \subfloat[\centering Distribution of solution for $p=1$]
    {{\includegraphics[width=0.45\columnwidth]{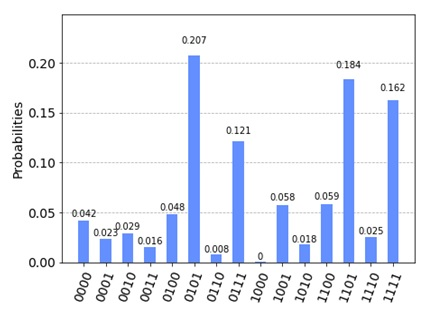} }} 
    \subfloat[\centering Distribution of solution for $p=2(NQ)^2$]
    {{\includegraphics[width=0.45\columnwidth]{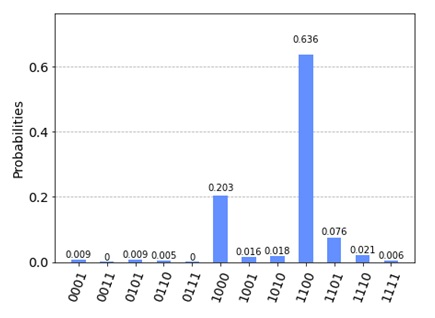} }} 
    \\
    \subfloat[\centering Iteration curve for $p=2(NQ)^2$]
    {{\includegraphics[width=0.48\columnwidth]{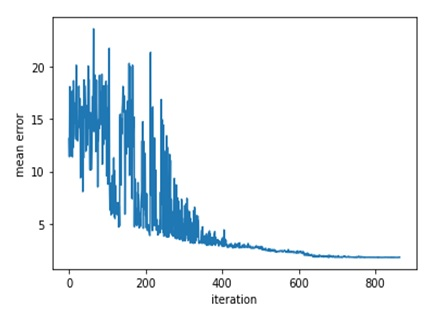} }}%
    \subfloat[\centering Performance Table]
    {{\includegraphics[width= 0.48\columnwidth]{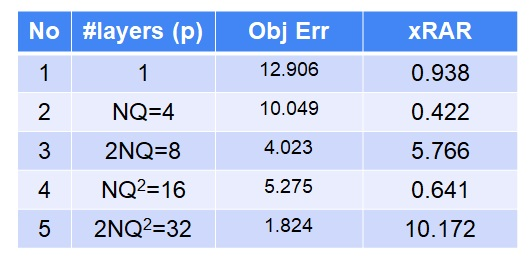} }}%
    
    \caption{Uniform k-Body with Non-Uniform Coefficients}%
    \label{FIG_kbody_non_uniform_coeffs}%
\end{figure*}
