# Supplementary material for: A Quantum Approximate Optimization Method For Finding Hadamard Matrices
Source: arXiv:2408.07964 source file (2024-10-13)
Supplement: Supplementary file 2 [file AppendixA.tex]

%\appendix
%\newpage
\section{Representative problems for each $k$-body cases}
In this section, we will evaluate and validate each of the k-body circuits with a simple problem of finding low order H-matrix before employing them into the full problem. The prototypical problem is finding a 2-order H-matrix, where the unknown entries will subsequently be increased to represent the increasing number of interaction $k$ for the $k$-body terms.

%\subsubsection{Elementary cases}
\subsection{1-body}
% -- 1-Body, QAOA ------
\begin{figure*}[h!]
    \centering
    \subfloat[\centering A quantum circuit for 2-qubits QAOA problem]
    {{\includegraphics[width=0.6\columnwidth]{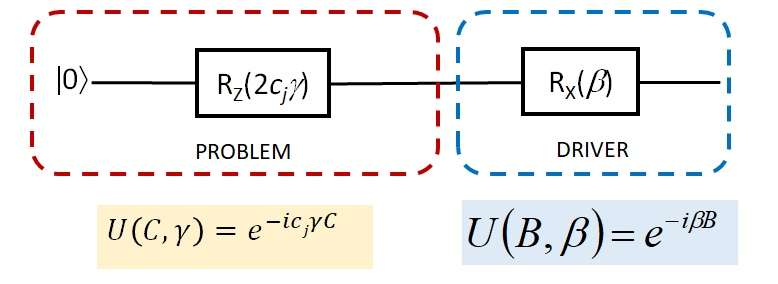} }}%
    %\qquad
    \\
    \subfloat[\centering Realized Quantum Circuit in Qiskit]
    {{\includegraphics[width=0.45\columnwidth]{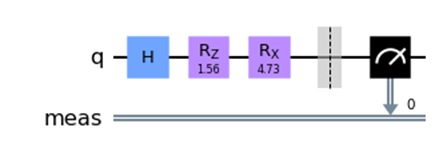} }} %
    \subfloat[\centering Distribution of solution]
    {{\includegraphics[width=0.45\columnwidth]{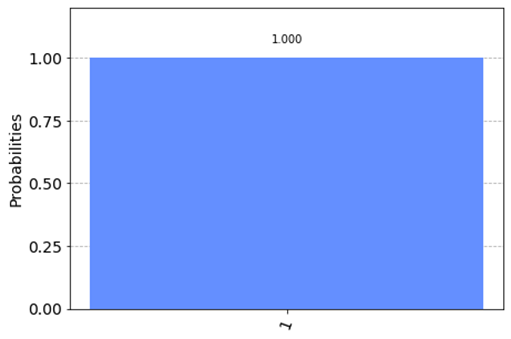} }} %
    %%--
    \caption{ Quantum Circuit for 1-body Interaction}%
    \label{FIG_1BODYX}%
\end{figure*}
The first case to consider is the problem involving only 1-body terms. A representative problem of finding 2-order H-matrix with 1 unknown can be formulated as follows
\begin{equation}
    \nonumber
    \begin{pmatrix}
        1 & 1  \\
        1 & s_1
    \end{pmatrix}
\end{equation}

The related energy function as formulated in Eq.(\ref{EQ_QAOA_problem}) is then given by

\begin{equation}
    E=2(1+s_1)
    \label{EQ_1body_hsearch}
\end{equation}
whose corresponding Hamiltonian is 
\begin{equation}
    \hat{H}\left( \hat{\sigma}\right)=2\left(1+\hat{\sigma}^z_{1}\right) 
    \label{EQ_1body_hsearch_hamiltonian}
\end{equation}
It is obvious that the solution will be $s_1 = -1$, which in the binary variable domain is equal to "1" (remind that the spin-to-binary variable transform is: $"0" \leftrightarrow  1, "1" \leftrightarrow -1$). The corresponding QAOA circuit can be constructed after insertion of driver Hamiltonian represented as an X-rotation of angle $\beta$, which is shown in Fig.\ref{FIG_1BODYX}(a). After constructing the circuit and running the program, we obtain the results shown in Fig. \ref{FIG_1BODYX} (b) and (c).

We can calculate the performance of this algorithm as follows. Since there is only one variable, a random algorithm will output a single bit string, therefore are two possibilities of the output, which are "0" and "1". The probability of the solution in the random algorithm is $P_R=\frac{1}{2}=0.5$. On the other hand, the quantum algorithm gives one correct answer so that $P_A=1.0$ as shown in the histogram. Accordingly, we have $xRR=\frac{P_A}{P_R} = 2$.

\subsection{2-body}
% -- 2-Body, QAOA ------
\begin{figure*}[h!]
    \centering
    \subfloat[\centering A quantum circuit for 2-qubits QAOA problem]
    {{\includegraphics[width=0.6\columnwidth]{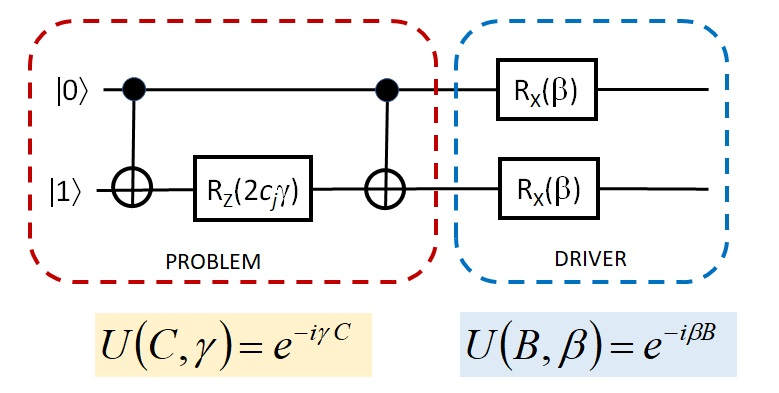} }}%
    %\qquad
    \\
    \subfloat[\centering Realized Quantum Circuit in Qiskit]
    {{\includegraphics[width=0.45\columnwidth]{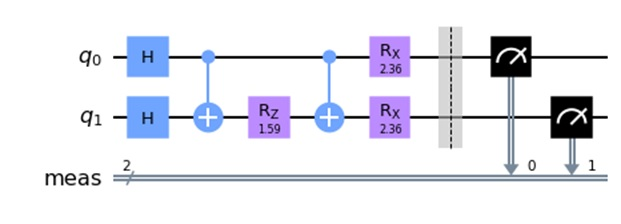} }} %
    \subfloat[\centering Distribution of solution]
    {{\includegraphics[width=0.45\columnwidth]{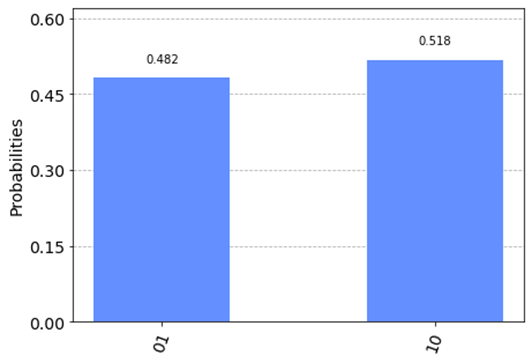} }} %
    \caption{QAOA circuits and simulation results of 2-qubits problem}%
    \label{FIG_2BODYX}%
\end{figure*}
%
% --- need related simulations on quantum simulator ---
The prototypical problem for a 2-body case can be formulated similarly, but now we have two variables $s_1, s_2$. We can formulate the searched matrix as follows
\begin{equation}
    \nonumber
    \begin{pmatrix}
        1 & s_1  \\
        1 & s_2
    \end{pmatrix}
\end{equation}

The energy function related to this problem is therefore
\begin{equation}
    E=(s_1+s_2)^2 = 2(1+s_1s_2)
    \label{EQ_2body_hsearch}
\end{equation}
whose corresponding Hamiltonian is 
\begin{equation}
    \hat{H}\left( \hat{\sigma}\right)=2\left(1+\hat{\sigma}^z_{1}\hat{\sigma}^z_{2} \right) 
    \label{EQ_2body_hsearch_hamiltonian}
\end{equation}
the simplification is obtained since we know that $s_i \in {-1,1}$ implying $s_i^2=1$. Obviously, the solution in the binary form will be either "01" or "10". The quantum circuit for this problem is given by Fig. \ref{FIG_2BODYX} (a). 

Running the circuit into a simulator of quantum processor gives the following result displayed in Fig.\ref{FIG_2BODYX} (b) and its histogram in (c). The histogram of the simulation results shows that the solution is distributed almost equally into "01" and "10", as expected. Since the output is a 2-bit strings and there are 2 valid solutions, the probability of the solution by the random algorithm is $P_R=\frac{2}{4}=\frac{1}{2}=0.5$. From Fig. Fig.\ref{FIG_2BODYX} (c) we have $P_A=0.482+0.518 = 1.0$; therefore $xRR=\frac{1}{0.5}=2$.

\subsection{3-body}
% -- 3-Body, QAOA ------
\begin{figure*}[h!]
    \centering
    \subfloat[\centering A quantum circuit for 3-qubits QAOA problem]
    {{\includegraphics[width=0.6\columnwidth]{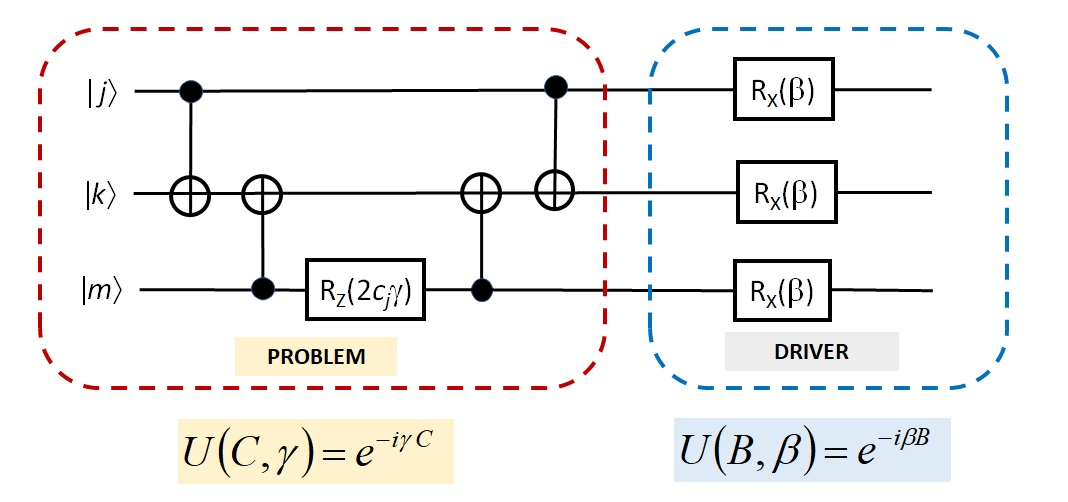} }}%
    %\qquad
    \\
    \subfloat[\centering Realized Quantum Circuit in Qiskit]
    {{\includegraphics[width=0.45\columnwidth]{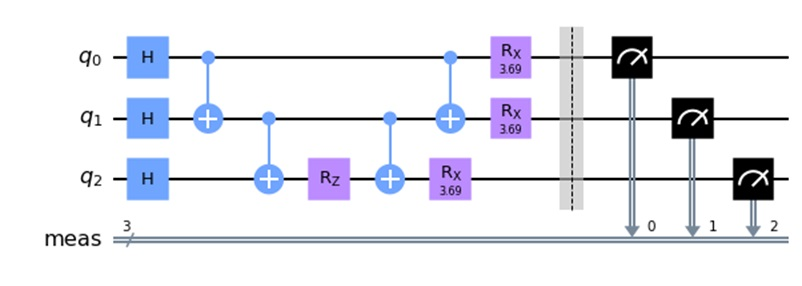} }} 
    \subfloat[\centering Distribution of solution]
    {{\includegraphics[width=0.45\columnwidth]{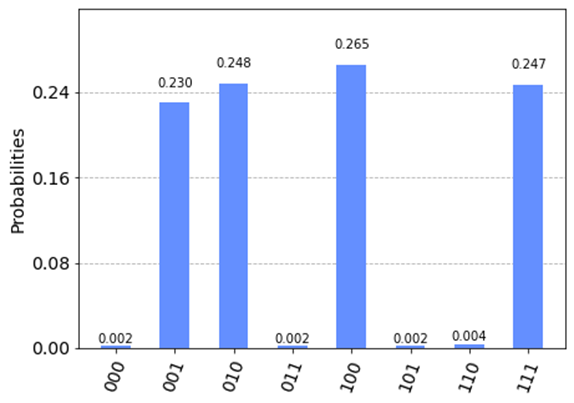} }} %
    %% -- 
    \caption{QAOA circuits and simulation results of 3-qubits problem}%
    \label{FIG_3BODYX}%
\end{figure*}
The 3-body prototypical problem can be represented by 3-unknown entries with corresponding variables $s_1, s_2, s_3$ in the 2-order H-matrix as follows

\begin{equation}
    \nonumber
    \begin{pmatrix}
        1 & s_1  \\
        s_2 & s_3
    \end{pmatrix}
\end{equation}

The related energy function can be computed similarly, which gives the following expression 
\begin{equation}
    E=(s_1+s_2s_3)^2 = 2(1+s_1s_2s_3)
    \label{EQ_3body_hsearch}
\end{equation}
whose corresponding Hamiltonian is 
\begin{equation}
    \hat{H}\left( \hat{\sigma}\right)=2\left(1+\hat{\sigma}^z_{1}\hat{\sigma}^z_{2} \hat{\sigma}^z_{3} \right) 
    \label{EQ_3body_hsearch_hamiltonian}
\end{equation}
The quantum circuit for this problem is displayed in Fig. \ref{FIG_3BODYX} (a). Then, we run the circuit in quantum simulator and get the following results shown in Fig.\ref{FIG_3BODYX} (b) and  (c). The histogram in (c) shows the peak distributions into 4 cases corresponding with solution of "001", "010", "100", and "111". Considering bit "1" represents "-1" spin-value, all of the peaks are correct solutions. Since the output is a 3-length bitstrings, the probability of the solution in a random algorithm is $P_R=4\frac{1}{8}=\frac{1}{2}=0.5$, whereas the probability of the solution by the quantum algorithm as shown in the histogram is $P_A=0.230+0.248+0.265+0.247=0.99$. Therefore, the performance metric is $xRR=\frac{0.99}{0.5}= 1.98$.

% -- 4-Body, QAOA ------
\begin{figure*}[h!]
    \centering
    \subfloat[\centering A quantum circuit for 4-qubits QAOA problem]
    {{\includegraphics[width=0.6\columnwidth]{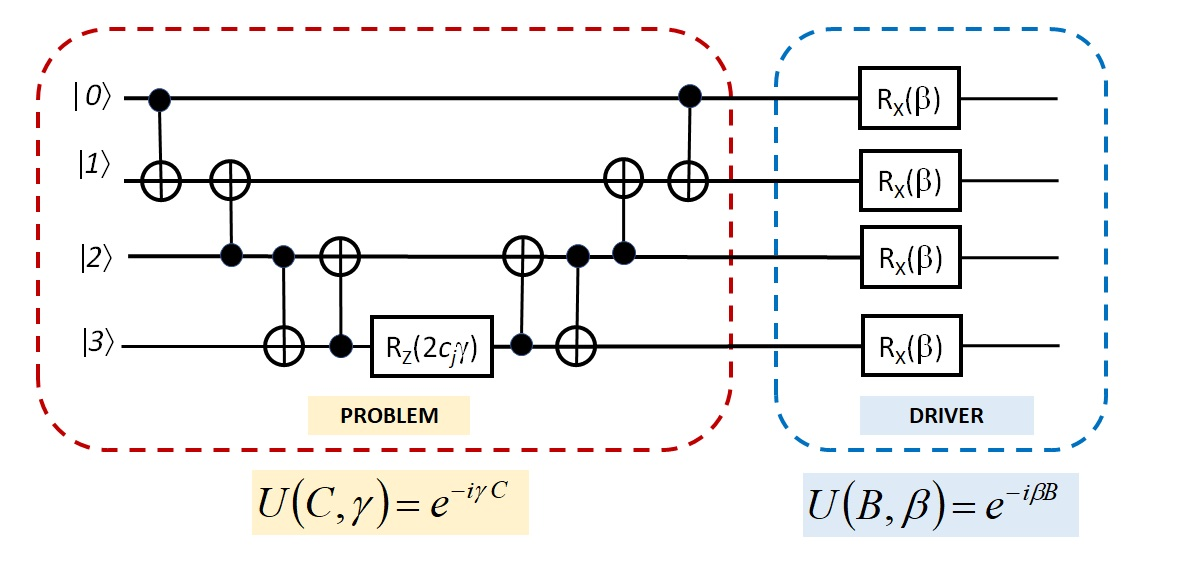} }}%
    %\qquad
    \\    
    \subfloat[\centering Realized Quantum Circuit in Qiskit]
    {{\includegraphics[width=0.45\columnwidth]{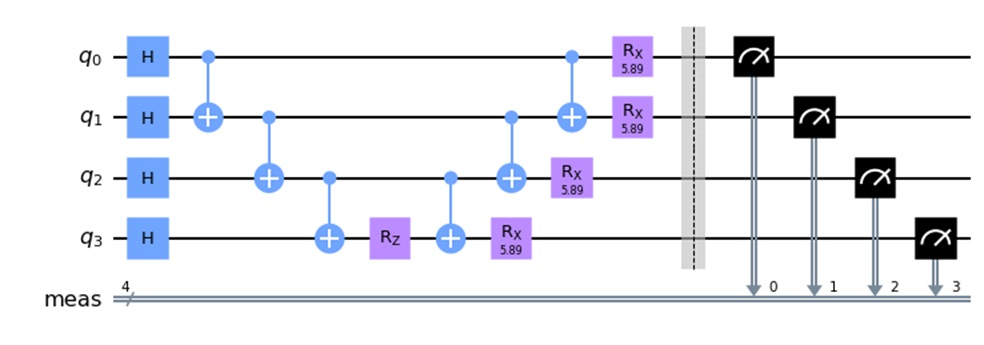} }} 
    \subfloat[\centering Distribution of solution]
    {{\includegraphics[width=0.45\columnwidth]{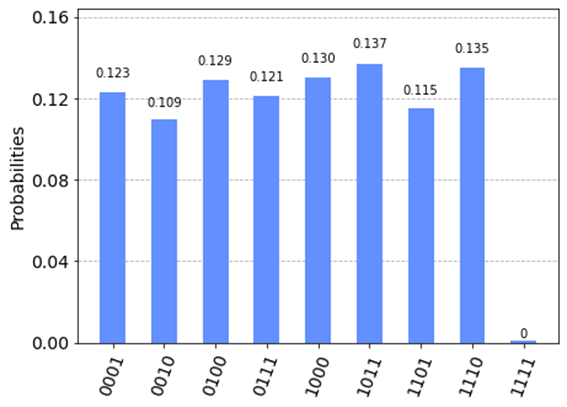} }} %
    \caption{QAOA circuits and simulation results of 4-qubits problem}%
    \label{FIG_4BODYX}%
\end{figure*}

\subsection{4-body}
%The last case is 4-body interactions. 
The matrix related to 4-body interaction is given as follows,
%We did the experiment with two cases, i.e., 4-body embedded in a 2-order H-matrix and in a 4-order H-matrix. 
%For the first case, the 2-order H-matrix is given as follows
\begin{equation}
    \nonumber
    \begin{pmatrix}
        s_1 & s_3  \\
        s_2 & s_4
    \end{pmatrix}
\end{equation}
with energy related function is given by
\begin{equation}
    E=(s_1s_3+s_2s_4)^2 = 2(1+s_1s_2s_3s_4)
    \label{EQ_4body_hsearch}
\end{equation}
whose corresponding Hamiltonian is given by
\begin{equation}
    \hat{H}\left( \hat{\sigma}\right)=2\left(1+\hat{\sigma}^z_{1}\hat{\sigma}^z_{2} \hat{\sigma}^z_{3}\hat{\sigma}^z_{4} \right) 
    \label{EQ_4body_hsearch_hamiltonian}
\end{equation}
The quantum circuit for this problem is given by Fig. \ref{FIG_4BODYX} (a).

We run the circuit in quantum simulator and get the following results shown in Fig.\ref{FIG_4BODYX}(b) and (c). The histogram in (c) shows the peak distributions into 4 cases corresponding with solution of "0001", "0010", "0100", "0111", "1000", "1011", "1101", and "1110", all of them are correct solutions. The probability of correct solution in a random algorithm will be $P_R=8\frac{1}{2^4}=0.5$, whereas the probability of the quantum algorithm is $P_A=0.123+0.109+0.129+0.121+0.130+0.137+0.115+0.135=0.999$. Therefore, the performance metric is $xRR=\frac{P_A}{P_R} = \frac{0.999}{0.5}=1.998$.
