# Supplementary material for: A Quantum Approximate Optimization Method For Finding Hadamard Matrices
Source: arXiv:2408.07964 source file (2024-10-13)
Supplement: Supplementary file 3 [file AppendixB.tex]

\section{Cascaded $k$-body cases}
The previous subsection presents experiments of individual $k$-body cases, which are the simplest case involving Problem Hamiltonian with only one term. In this subsection, we present the experiments results when the terms are unified. Some sub cases will be considered, which are: (a) uniform $k$-body and with uniform coefficients, (b) uniform $k$-body with non-uniform coefficients, and (c) mixed $k$-body. We minimize the mean error of the objective function by using the COBYLA (Constrained Optimization BY Linear Approximatio) method provided in Pyhton package. The initial values of the parameters $\{\gamma, \beta \}$ are set at random.

% -- uniform 2-body, uniform coeffs------
\begin{figure*}[h!]
    \centering
    \subfloat[\centering Iteration curve for $p=1$]
    {{\includegraphics[width=0.45\columnwidth]{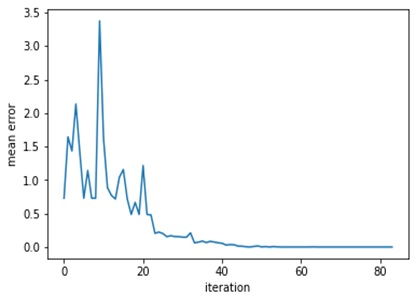} }}%
    %\qquad    
    \subfloat[\centering Distribution of solution for $p=4$]
    {{\includegraphics[width=0.45\columnwidth]{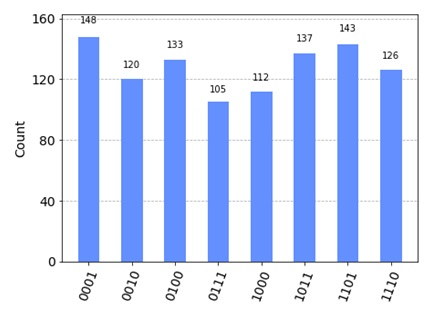} }} 
    \\
    \subfloat[\centering Quantum Circuit $p=1$]
    {{\includegraphics[width= 1.0\columnwidth]{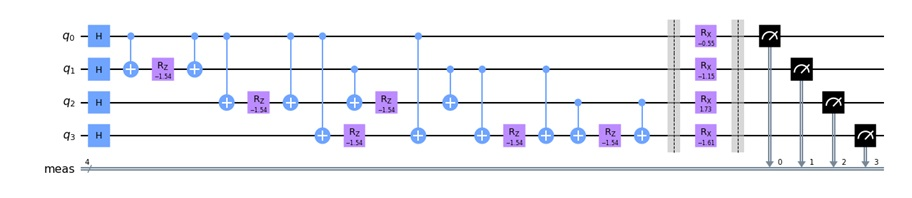} }}%
    
    \caption{Uniform 2-Body with Uniform Coefficients}%
    \label{FIG_2body_uniform_coeffs}%
\end{figure*}
%

%/////////////////////////////////////////////////////////////
\subsection{Case-1: 2-body terms with uniform coefficients}
%/////////////////////////////////////////////////////////////
The Hamiltonian terms in this case are similar to the max-cut problem. Here, we define a Hamiltonian that is not related particularly to the Hadamard matrix problem. All of the terms are 2-body interactions, which is given by

\begin{equation}
    H_P= s_0s_1 + s_0s_2 + s_0s_3 + s_1s_2 + s_1s_3 + s_2s_3
    \label{EQ_2body_uniform_coeffs}
\end{equation}

Since there ae 4 binary variables, the number of total possible output is 16. An exhaustive check shows that there are 8 bit strings of correct solutions, which are $\{0001, 0010, 0100, 0111, 1000, 1011, 1101, 1110\}$. This give the probability of random algorithm $P_R=\frac{8}{16}=\frac{1}{2}$. 

We found that running QAOA on a simulator with $p=1$ is sufficient to find all solutions. The simulation results are displayed in Fig.\ref{FIG_2body_uniform_coeffs}, with (a) the iteration curve, (b) distribution of solution, and (c) quantum circuit of the problem. The quantum circuit shown in (c) is similar to the QAOA of maxcut problems [REF-IBM-qiskit-book]. The final objective functions reach the absolute minimum of $0.000$ and all of $1024$ shots gives a correct solutions which corresponds to $P_A=1.000$. Accordingly, the performance is $xRAR=\frac{P_A}{P_R}=2.000$.

% -- uniform 2-body, non-uniform coeffs------
\begin{figure*}[h!]
    \centering
    \subfloat[\centering Iteration curve for $p=1$]
    {{\includegraphics[width=0.45\columnwidth]{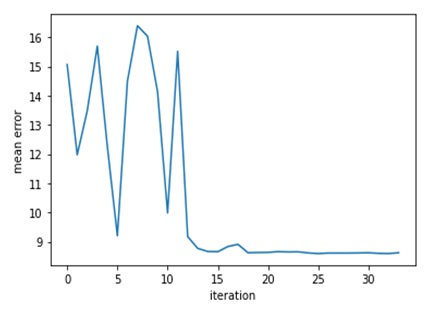} }}%
    %\qquad    
    \subfloat[\centering Distribution of solution for $p=1$]
    {{\includegraphics[width=0.45\columnwidth]{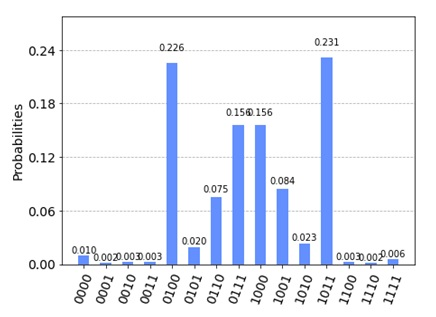} }} 
    \\
    \subfloat[\centering Quantum Circuit $p=1$]
    {{\includegraphics[width= 1.0\columnwidth]{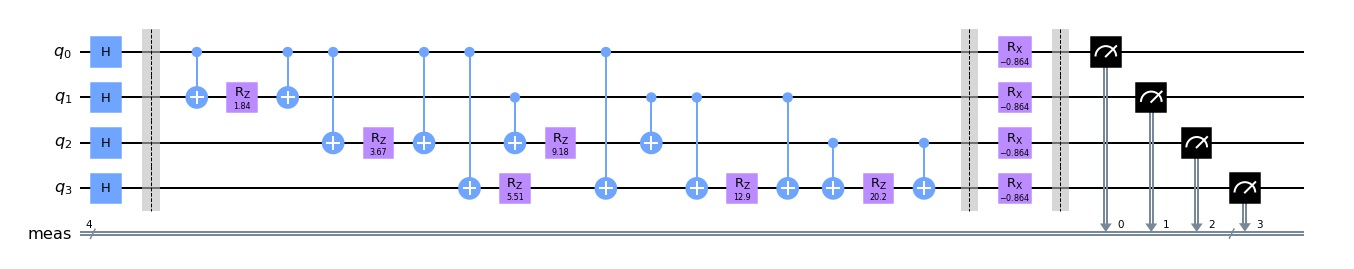} }}%
    
    \caption{Uniform 2-Body with Non-Uniform Coefficients}%
    \label{FIG_2body_non_uniform_coeffs_01}%
\end{figure*}
%
%/////////////////////////////////////////////////////////////
\subsection{Case-2: 2-body with non-uniform coefficients}
%/////////////////////////////////////////////////////////////
In this experiment, the Hamiltonian of the problem is given by the following 
\begin{equation}
    H_P= s_0s_1 + 2s_0s_2 + 3s_0s_3 + 5s_1s_2 + 7s_1s_3 + 11s_2s_3 -3
    \label{EQ_2body_non_uniform_coeffs}
\end{equation}
The constant $3$ in this equation is an offset that makes the absolute minimum value of $H_P$ equal to zero. This equation Eq.(\ref{EQ_2body_uniform_coeffs}) is slightly different from Eq.(\ref{EQ_2body_non_uniform_coeffs}), all terms are two-bodies but with several different  coefficients in the later. The total number of possible output is also 16, but the correct solutions is 2; which are $\{0100, 1011\}$ this gives $P_R=\frac{1}{8}$. 

We do the experiment by increasing the number of layers $p$. The results are displayed in Fig. \ref{FIG_2body_non_uniform_coeffs_01} and Fig. \ref{FIG_2body_non_uniform_coeffs_02}, which shows increasing performance in terms of increasing xRAR and decreasing objective error. The table in Fig. \ref{FIG_2body_non_uniform_coeffs_02} (c) clearly shows increasing performance with increasing number of layers.

% -- uniform 2-body, non-uniform coeffs:: FIG-2------
\begin{figure*}[h!]
    \centering
    \subfloat[\centering Iteration curve for $p=2NQ^2$]
    {{\includegraphics[width=0.45\columnwidth]{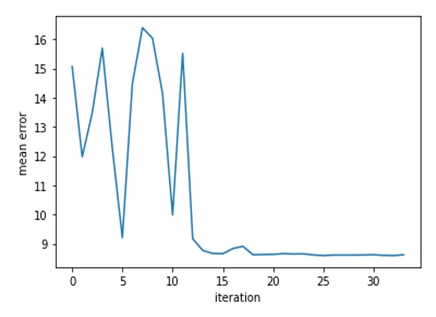} }}%
    %\qquad    
    \subfloat[\centering Distribution of solution for $p=1$]
    {{\includegraphics[width=0.45\columnwidth]{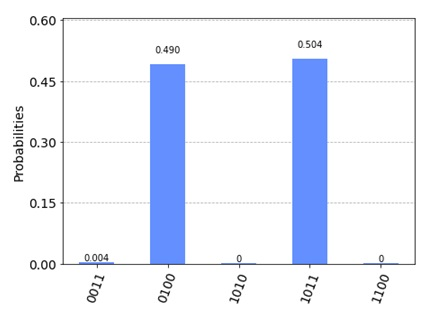} }} 
    \\
    \subfloat[\centering Performance Table]
    {{\includegraphics[width= 0.5\columnwidth]{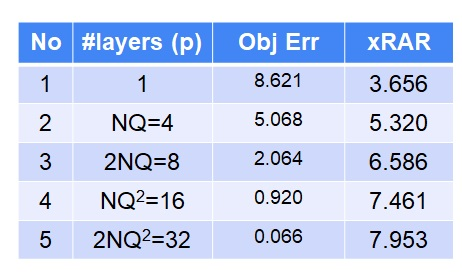} }}%
    
    \caption{Uniform 2-Body with Non-Uniform Coefficients: high layer number and table of performance}%
    \label{FIG_2body_non_uniform_coeffs_02}%
\end{figure*}

\subsection{Case-3: mixed $k$-body, uniform coefficients}
In this case, we have the following problem Hamiltonian
\begin{equation}
    \label{EQ_mixed_k_body_uniform_coeffs_hamiltonian}
    H_P= s_0 + s_1 + s_2 + s_0s_1 + s_1s_2 + s_1s_2s_3 + s_0s_1s_2s_3-1
\end{equation}

There are 4 valid bit string solutions, which are $\{0101, 0110, 1000, 1001\}$, so that $P_R=\frac{1}{4}$. Simulation results are shown in Fig.\ref{FIG_kbody_uniform_coeffs}. The distribution in (b) shows dominant probability on the solutions, while the table in (c) shows increasing performance with increasing $p$.

% -- mixed k-body, uniform coeffs
\begin{figure*}[h!]
    \centering
    \subfloat[\centering Distribution of solution for $p=1$]
    {{\includegraphics[width=0.45\columnwidth]{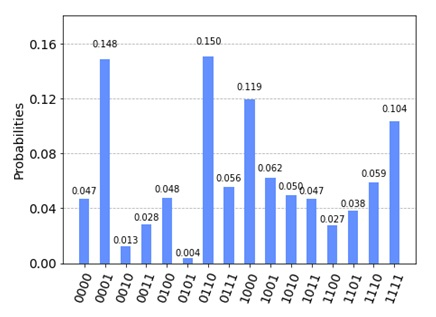} }} 
    \subfloat[\centering Distribution of solution for $p=2(NQ)^2$]
    {{\includegraphics[width=0.45\columnwidth]{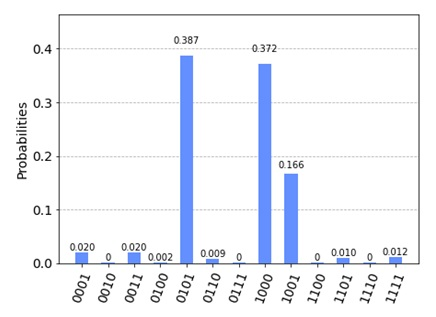} }} 
    \\
    \subfloat[\centering Iteration curve for $p=2(NQ)^2$]
    {{\includegraphics[width=0.48\columnwidth]{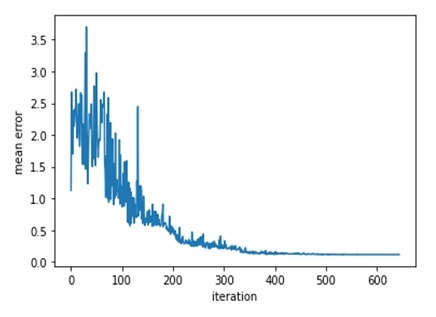} }}%
    %\qquad    
    \subfloat[\centering Performance Table]
    {{\includegraphics[width= 0.48\columnwidth]{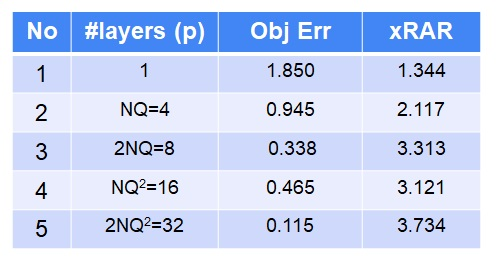} }}%
    \caption{Mixed k-Body with Uniform Coefficients}%
    \label{FIG_kbody_uniform_coeffs}%
\end{figure*}

\subsection{Case-4: mixed $k$-body, non-uniform coefficients}
The problem Hamiltonian for mixed $k$-body with non uniform coefficients is as follows,
\begin{equation}
    \label{EQ_mixed_k_body_uniform_coeffs_hamiltonian}
    H_P= s_0 + 2s_1 + 3s_2 + 5s_0s_1 + 7s_1s_2 + 11s_1s_2s_3 + 13s_0s_1s_2s_3
\end{equation}

There is only one valid bit string for this problem, which is $1100$, so that the probability of random algorithm is $P_R=16$. Some of the simulation results are displayed in Fig.\ref{FIG_kbody_non_uniform_coeffs}. In part (b) and (c), we observe re-concentration of distribution toward the solution at higher value of $p$. The performance table in (d) shows that increasing $p$ tends to iprove the performance, although at some value of $p$ it can reduced.

% -- mixed k-body, non-uniform coeffs
\begin{figure*}[h!]
    \centering
    \subfloat[\centering Distribution of solution for $p=1$]
    {{\includegraphics[width=0.45\columnwidth]{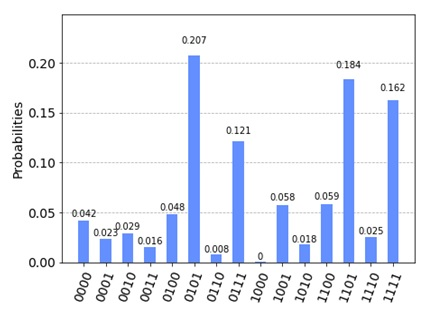} }} 
    \subfloat[\centering Distribution of solution for $p=2(NQ)^2$]
    {{\includegraphics[width=0.45\columnwidth]{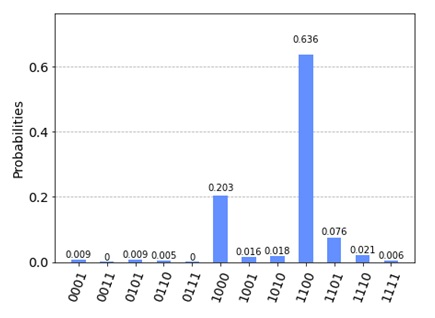} }} 
    \\
    \subfloat[\centering Iteration curve for $p=2(NQ)^2$]
    {{\includegraphics[width=0.48\columnwidth]{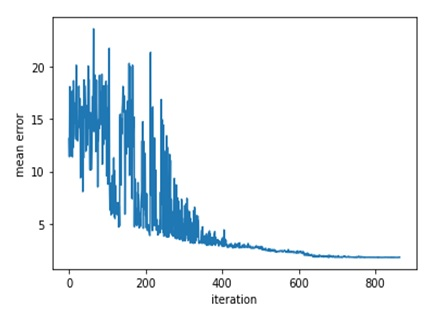} }}%
    \subfloat[\centering Performance Table]
    {{\includegraphics[width= 0.48\columnwidth]{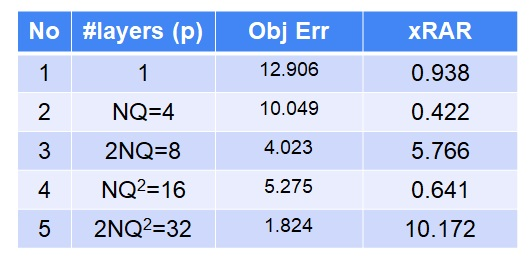} }}%
    
    \caption{Uniform k-Body with Non-Uniform Coefficients}%
    \label{FIG_kbody_non_uniform_coeffs}%
\end{figure*}
